# Supplementary material for: A Simultaneous Decoding Approach to Joint State and Message Communications
Source: arXiv:2501.11133 source file (2025-02-13)
Supplement: Supplementary file 1 [file deg-bc-scc-commonly.tex]

Again, we only provide the proof for the causal case, and the extension to the strictly causal case is simply done by removing $X$'s dependency on $S_T$. The proof of achievability is finished in Appendix~\ref{app:deg-bc-scc} and here we only need to show that for all required possible $D_1$ with $D_1^{(n)}\le D_1$, the rate tuple $(R_0, R_1, R_2)$ cannot be beyond the region defined in $\calR(\pddcf{D_1}{\infty}|_{Y_2'= \varnothing})$. We define the following auxiliary random variables:
\begin{equation}
\begin{split}
    W_i &= (M_1, M_2, S_T^{i-1}),\\
    U_{2,i} &= (M_2, Z_1^{i-1}, Z_2^{i-1}),\\
    U_{1,i} &= (W_i, Y'^{i-1}) = (M_1, M_2, S_T^{i-1}, Y'^{i-1}),\\
    V_{1,i} &= Z_{1,i+1}^n,
\end{split}
\end{equation}
and it is verified that 
\begin{equation*}
\begin{split}
    &P_{S_iS_{T,i}U_{1,i}U_{2,i}V_{1,i}X_iZ_{1,i}Z_{2,i}Y'_i}(s_i,s_{T,i}, u_{1,i}, u_{2,i}, v_{1,i}, x_i, z_{1,i}, z_{2,i}, y_i)=P_S(s_i)P_{S_T|S}(s_{T,i}|s_i)P_{U_{2,i}}(u_{2,i}) \\
    &\Hquad \cdot P_{U_{1,i}|U_{2,i}}(u_{1,i}|u_{2,i}) \mathbbm{1}\{x_i=g_{e,i}(u_{1,i}, s_{T,i})\} P_{Z_1Z_2|XS}(z_{1,i},z_{2,i}|x_i, s_i) \mathbbm{1}\{y'_i=\phi_1(z_{1,i})\}P_{V_i|U_{1,i}S_{T,i}Y'_i}(v_{1,i} | u_{1,i}, s_{T,i}, y'_i).\\
\end{split}
\end{equation*}
Since the cardinality of $\calU_{1,i}=\calM_1 \times \calM_2 \times \calS_T^{i-1} \times \calY'^{i-1}$ varies for different $i$, we can define a function $g_e$ independent of $i$ and defined on $\bigcup_i \calU_{1,i} \times \calS_T$ with $g_e(u_i, s_{T,i}) = g_{e,i}(u_i,s_{T,i})=x_i$. The estimator $h_{1,i}(Z_1^n)$ can be replaced by $h^*_{1,i}(U_{1,i}, U_{2,i}, V_{1,i}, Z_{1,i})$ because
\begin{equation}
    \expcs{}{d_1(S_i, h_{1,i}(Z_1^n))} \ge \expcs{}{d_1(S_i, h^*_{1,i}(U_{1,i}, U_{2,i}, V_{1,i}, Z_{1,i}))}
\end{equation}
due to the Markov chain $S_i - (U_{1,i}, U_{2,i}, V_{1,i}, Z_{1,i}) - Z_1^{i-1}$ and Lemma~\ref{lemma:markovest}. Introducing a time-sharing random variable $Q$ that is uniformly distributed over $[n]$ and independent of all the other random variables, and redefining $U_1=U_{1,Q}$, $U_2=(Q,U_{2,Q})$, $V_1=V_{1,Q}$, $S = S_Q$, $S_T=S_{T,Q}$, $X=X_Q$, $Z_1=Z_{1,Q}$, $Z_2=Z_{2,Q}$, $Y'=Y'_Q$, $\hS_1=\hS_{1,Q}$, $h_1^*(U_1, U_2, V_1, Z_1) = h^*_{1,Q}(U_{1,Q}, U_{2,Q}, V_{1,Q}, Z_{1,Q})$ it can be shown that $(U_1, U_2, V_1, V_2, X, \hS_1,\hS_2) \in \pddcf{D_1}{\infty}$ with $V_2$ chosen arbitrarily and can be set to empty as it does not contribute to the decoding and estimation stages.

For decoder 2, we have
\begin{equation}\label{eq:r2converse}
    nR_2 -n\epsilon_n \le I(M_2; Z_2^n) \le \sum_{i=1}^n I(M_2, Z_2^{i-1}; Z_{2,i}) \le \sum_{i=1}^n I(U_{2,i}; Z_{2,i}) = nI(U_2; Z_2)
\end{equation}
due to the Fano's inequality. We can also identify the equality
\begin{equation}
    I(Z_1^n; S_{T,i} | W_i) = I(Z_1^n, \hS_{1,i}; S_{T,i} | W_i)= I(\hS_{1,i}; S_{T,i} | W_i) + I(Z_1^n; S_{T,i} | W_i, \hS_{1,i}),
\end{equation}
such that
\begin{subequations}\label{eq:r1converse}
\begin{align}
    nR_1 & + \sum_{i=1}^n I(\hS_{1,i}; S_{T,i} | W_i) - n\epsilon_n\\
    &\le I(M_1; Z_1^n | M_2) + \sum_{i=1}^n \brsq{I(Z_1^n; S_{T,i} | W_i)-I(Z_1^n; S_{T,i} | W_i, \hS_{1,i})}\\
    &= I(M_1; Z_1^n | M_2) + I(Z_1^n; S_{T}^n | M_1,M_2) - \sum_{i=1}^nI(Z_1^n; S_{T,i} | W_i, \hS_{1,i})\\
    &= I(M_1, S_T^n; Z_1^n | M_2) - \sum_{i=1}^nI(Z_1^n; S_{T,i} | W_i, \hS_{1,i})\\
    &= \sum_{i=1}^n \brsq{I(M_1, S_T^n; Z_{1,i} | M_2, Z_1^{i-1}, Z_2^{i-1}) - I(Z_1^n; S_{T,i} | W_i, \hS_{1,i})}\label{subeq:bc-converse-1}\\
    &= \sum_{n=1}^n \brsq{H(Z_{1,i}| U_{2,i}) - H(Z_{1,i}| U_{1,i},U_{2,i},S_{T,i}) - I(Z_1^n; S_{T,i} | W_i, \hS_{1,i})}\label{subeq:bc-converse-3}\\
    &= \sum_{n=1}^n \brsq{I(Z_{1,i}; U_{1,i}, S_{T,i} | U_{2,i}) - I(Z_1^n; S_{T,i} | W_i, \hS_{1,i})}\\
    &= \sum_{n=1}^n \brsq{I(Z_{1,i}; U_{1,i} | U_{2,i}) + I(Z_{1,i}; S_{T,i} | U_{1,i}, U_{2,i}) - I(Z_1^n; S_{T,i} | W_i, \hS_{1,i})}\\
    &\le \sum_{n=1}^n \brsq{I(Z_{1,i}; U_{1,i} | U_{2,i}) + H(S_{T,i}) - H(S_{T,i} | Z_{1,i},U_{1,i}, U_{2,i}) - H(S_{T,i} | W_i, \hS_{1,i}) + H(S_{T,i} |U_{1,i}, U_{2,i}, V_{1,i}, Z_{1,i})}\label{subeq:bc-converse-2}\\
    &\le \sum_{n=1}^n \brsq{I(Z_{1,i}; U_{1,i} | U_{2,i}) - I(V_{1,i}; S_{T,i}|U_{1,i}, U_{2,i}, Z_{1,i}) + I(S_{T,i}; W_i, \hS_{1,i})},
    % &= \sum_{n=1}^n \brsq{I(Z_{1,i}; U_{1,i} | U_{2,i}) - I(V_{1,i}; S_{T,i}, Y'_i|U_{1,i}, U_{2,i}, Z_{1,i}) + I(S_{T,i}; \hS_{1,i} |W_i)}\label{subeq:bc-converse-3},
\end{align}
\end{subequations}
where \eqref{subeq:bc-converse-1} and \eqref{subeq:bc-converse-2} follow since the channel is degraded, \eqref{subeq:bc-converse-3} holds because $Y'_i$ is a deterministic function of $Z_{1,i}$. Subsequently, 
\begin{subequations}
\begin{align}
    R_1- \epsilon_n &\le \frac{1}{n}\sum_{n=1}^n \brsq{I(Z_{1,i}; U_{1,i} | U_{2,i}) - I(V_{1,i}; S_{T,i}|U_{1,i}, U_{2,i}, Z_{1,i})}\\
    &=\frac{1}{n}\sum_{n=1}^n C_1\br{\expcs{}{d_1(S_i, h_{1,i}^*(U_{1,i}, U_{2,i}, V_{1,i}, Z_{1,i}))}}\\
    &\le C_1\br{\frac{1}{n}\sum_{n=1}^n \expcs{}{d_1(S_i, h_{1,i}^*(U_{1,i}, U_{2,i}, V_{1,i}, Z_{1,i}))}}\\
    &=C_1 \br{\expcs{}{d_1(S, h_1^*(U_1, U_2, V_1, Z_1))}}\\
    &\le C_1(D_1),
\end{align}
\end{subequations}
where $C_1(D_1)$ is the function of $R_1$ with respect to $D_1$ in $\calR(\pddcf{D_1}{\infty}|_{Y_2'= \varnothing})$, and is a non-decreasing concave function according to Proposition~\ref{prop:deg-bc-scc}. The sum rate should satisfy
\begin{subequations}
\begin{align}
    &n(R_1 + R_2 - 2\epsilon_n) + \sum_{i=1}^n I(\hS_{1,i}; S_{T,i} | W_i)\\
    &\quad \le I(M_2; Z_2^n) + I(M_1; Z_1^n|M_2) + \sum_{i=1}^n \brsq{I(Z_1^n; S_{T,i} | W_i)-I(Z_1^n; S_{T,i} | W_i, \hS_{1,i})}\\
    &\quad \le I(M_2; Z_1^n) + I(M_1; Z_1^n|M_2) + I(Z_1^n; S_{T}^n | M_1,M_2) - \sum_{i=1}^nI(Z_1^n; S_{T,i} | W_i, \hS_{1,i})\\
    &\quad = I(M_1, M_2; Z_1^n)+ I(Z_1^n; S_{T}^n | M_1,M_2) - \sum_{i=1}^nI(Z_1^n; S_{T,i} | W_i, \hS_{1,i})\\
    &\quad = I(M_1, M_2, S_T^n; Z_1^n) - \sum_{i=1}^nI(Z_1^n; S_{T,i} | W_i, \hS_{1,i})\\
    &\quad = \sum_{i=1}^n \brsq{I(M_1, M_2, S_T^n; Z_{1,i} | Z_1^{i-1}, Z_2^{i-1}) -I(Z_1^n; S_{T,i} | W_i, \hS_{1,i})}\\
    &\quad \le \sum_{i=1}^n \brsq{I(U_{1,i}, U_{2,i}, S_{T,i} ; Z_{1,i}) - I(Z_1^n; S_{T,i} | W_i, \hS_{1,i})}\\
    &\quad = \sum_{i=1}^n \brsq{ I(U_{1,i}, U_{2,i}; Z_{1,i}) + I(S_{T,i}; Z_{1,i} | U_{1,i}, U_{2,i}) -  I(Z_1^n; S_{T,i} | W_i, \hS_{1,i})}\\
    &\quad \le \sum_{i=1}^n \brsq{I(U_{1,i}, U_{2,i}; Z_{1,i}) + H(S_{T,i}) - H(S_{T,i}|U_{1,i}, U_{2,i}, Z_{1,i}) - H(S_{T,i}|W_i, \hS_{1,i}) + H(S_{T,i} | W_i, Z_1^n)}\\
    &\quad = \sum_{i=1}^n \brsq{I(U_{1,i}, U_{2,i}; Z_{1,i}) - I(V_{1,i} ; S_{T,i} | U_{1,i}, U_{2,i}, Z_{1,i}) + I(\hS_{1,i}; S_{T,i} | W_i)},
\end{align}
\end{subequations}
which is shown to hold automatically if \eqref{eq:r2converse} and \eqref{eq:r1converse} hold since the channel is degraded, and thus can be omitted.
